# Supplementary material for: Photon-mediated charge-exchange reactions between 39K atoms and 40Ca+ ions in a hybrid trap
Source: arXiv:2003.03430 ancillary file (2020-04-30)
Supplement: Supplementary file 1 [file Supplemental_CT.pdf]

# Supplemental Material: Photon-mediated charge-exchange reactions between $^{39}$K atoms and $^{40}$Ca$^+$ ions in a hybrid trap

Hui Li,[1] S. Jyothi,[2] Ming Li,[1] Jacek Kłos,[1,3] Alexander Petrov,[1,4] Kenneth R Brown,[2] and Svetlana Kotochigova[1,*]

[1] *Department of Physics, Temple University, Philadelphia, Pennsylvania 19122, USA*

[2] *Department of Electrical and Computer Engineering, Duke University, Durham, North Carolina 27708, USA*

[3] *Department of Chemistry and Biochemistry, University of Maryland, College Park, Maryland 20742, USA*

[4] *NRC, Kurchatov Institute PNPI, Gatchina, 188300, and Division of Quantum Mechanics, St. Petersburg State University, St. Petersburg, 199034, Russia*

## A. The electronic structure of the KCa$^+$ molecule

We have used the non-relativistic multi-reference configuration interaction (MRCI) method as implemented in the MOLPRO program package [1] to determine adiabatic Born-Oppenheimer potentials, non-adiabatic coupling matrix elements, and electronic transition dipole moments for the KCa$^+$ diatom. The inner-shell electrons for both K and Ca are described by the Stevens-Basch-Krauss-Jansien-Cundari (SBKJC) effective core potentials (ECP) [2], leaving only two valence electrons in the active space. The polarization of the effective cores is modeled via the core polarization potential (CPP) described in Ref. [3]. For the CPP, we use the static dipole polarizabilities of K$^+$ and Ca$^{2+}$, which are 5.472 a.u. [4] and 3.522 a.u. [5] respectively. Here, a.u. is an abbreviation for atomic unit. Müller/Meyer type cutoff functions are used with their exponents fitted to the asymptotic energies at large separation $R$, which yields the values 0.383 a.u. and 0.465 a.u. for K and Ca, respectively. For K we use the large 7s5p7d2f uncontracted Gaussian basis set from Ref. [6]. For Ca we use the contracted and optimized 9s7p6d/[7s6p6d] basis set from Ref. [7] augmented by three sets of f and one set of g polarization functions [8]. The contractions are specified in the square bracket. The multi-configurational self-consistent field (MCSCF) [9, 10] method is used to obtain molecular orbitals, followed by a full configuration interaction calculation (MRCI) with two-electron excitations.

Figure 1 shows the results of the MRCI calculations for six non-relativistic symmetries $^{2S+1}\Lambda^{\pm}$. The absolute ground state has $^1\Sigma^+$ symmetry.

Finally, we performed a comparison of our potentials with those of Refs. [11, 12]. The equilibrium separation $R_e$ and depth $D_e$ of the X$^1\Sigma^+$ potential agree to better than 1% and to 2%, respectively. The separation $R_e$ for most of the excited-state potentials agree to 1% with those of Ref. [12], however, the depths differ on average by 10% due to the sensitivity of this characteristic to the choice of basis set.

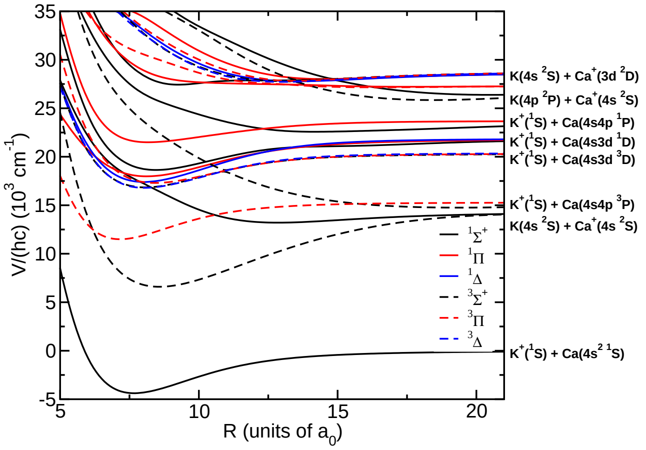


FIG. 1. Non-relativistic KCa$^+$ Born-Oppenheimer potential energy curves as functions of separation $R$. Potentials of all symmetries dissociating to the lowest eight atomic asymptotes are shown. Asymptotic atomic configurations are given on the right hand side of the graph. The zero of energy is at the K$^+$($^1$S) + Ca(4s$^2$ $^1$S) limit.

## B. Details on the quadrupole moment calculation

In our MRCI calculation of the quadrupole moment of the Ca (3d4p) $^3$P state the reference orbital were selected from the multi-reference self-consistent field calculation. Our active space consists of 4s, 4p, 4d, 5s, and 5p atomic orbitals of Ca. The calculation is performed with 10 electrons correlated and the inner 10 electrons kept in frozen core 1s, 2s, and 2p orbitals. The extended active space with higher n shell orbitals was necessary to include the state of interest in the roots of the CI expansion. The 3s and 3p orbitals were correlated but kept doubly occupied during the calculations. In order to reach the required excited state of the Ca atom we calculated 10 roots of the CI.

* skotoch@temple.edu

[1] H.-J. Werner, P. J. Knowles, G. Knizia, F. R. Manby, and M. Schütz, WIREs Comput. Mol. Sci. **2**, 242 (2012).
[2] W. J. Stevens, M. Krauss, H. Basch, and P. G. Jasien, Can. J. Chem. **70**, 612 (1992).
[3] W. Müller, J. Flesch, and W. Meyer, J. Chem. Phys. **80**, 3297 (1984).
[4] J. N. Wilson and R. M. Curtis, J. Phys. Chem. **74**, 187 (1970).
[5] H. Coker, J. Phys. Chem. **80**, 2078 (1976).
[6] M. Aymar and O. Dulieu, J. Chem. Phys. **122**, 204302 (2005).
[7] E. Czuchaj, M. Krosnicki, and H. Stoll, Mol. Phys. **98**, 419 (2000).
[8] E. Czuchaj, M. Krośnicki, and H. Stoll, Theor. Chem. Acc. **110**, 28 (2003).
[9] H. Werner and P. J. Knowles, J. Chem. Phys. **82**, 5053 (1985).
[10] P. J. Knowles and H.-J. Werner, Chem. Phys. Lett. **115**, 259 (1985).
[11] M. Śmiałkowski and M. Tomza, Phys. Rev. A **101**, 012501 (2020).
[12] W. Zrafi, H. Ladjimi, H. Said, H. Berriche, and M. Tomza, arXiv preprint arXiv:2003.02813 (2020).
